# Supplementary material for: Comparison of the charge-crystal and charge-glass state in geometrically frustrated organic conductors studied by fluctuation spectroscopy
Source: arXiv:2202.05602 source file (2022-02-11)

$\theta_o$ -type

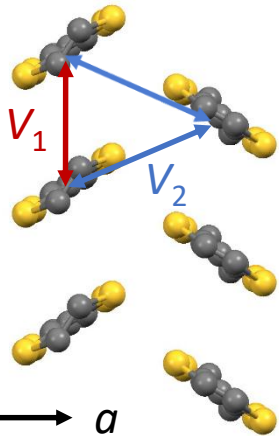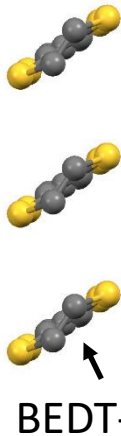

$\theta_m$ -type

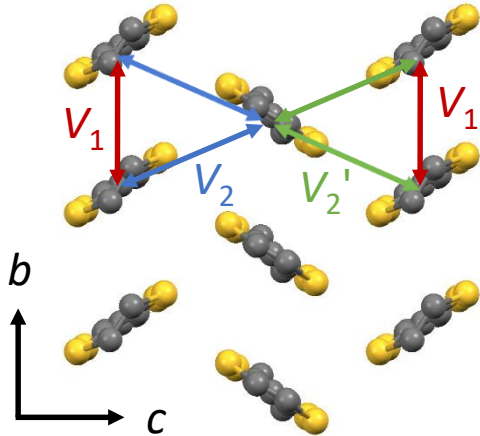

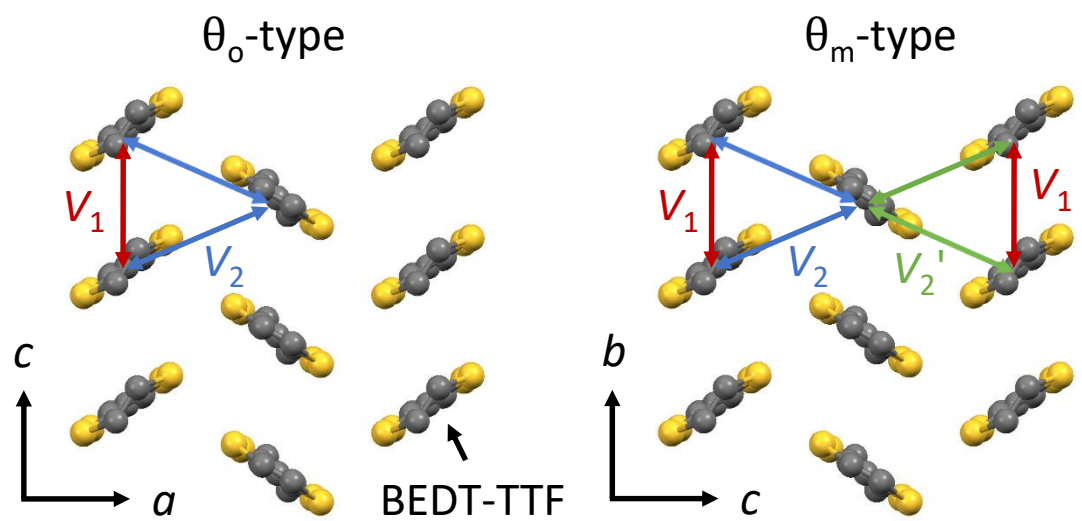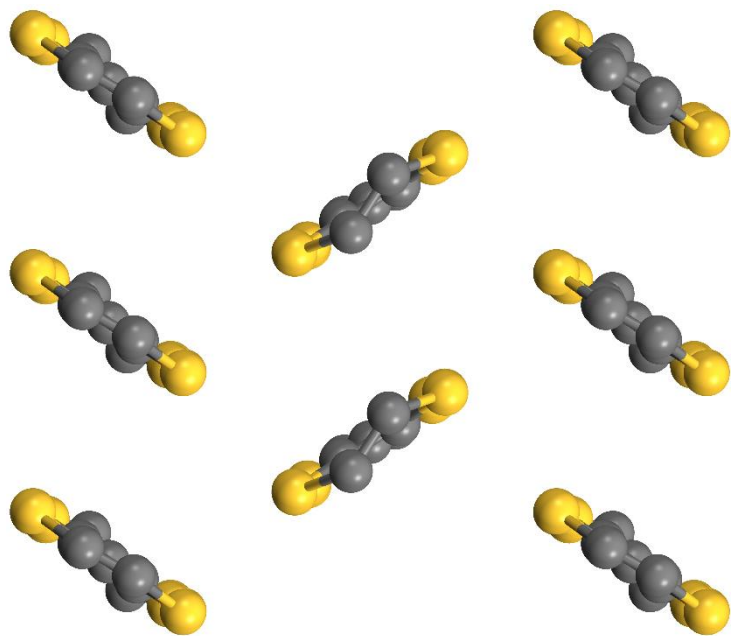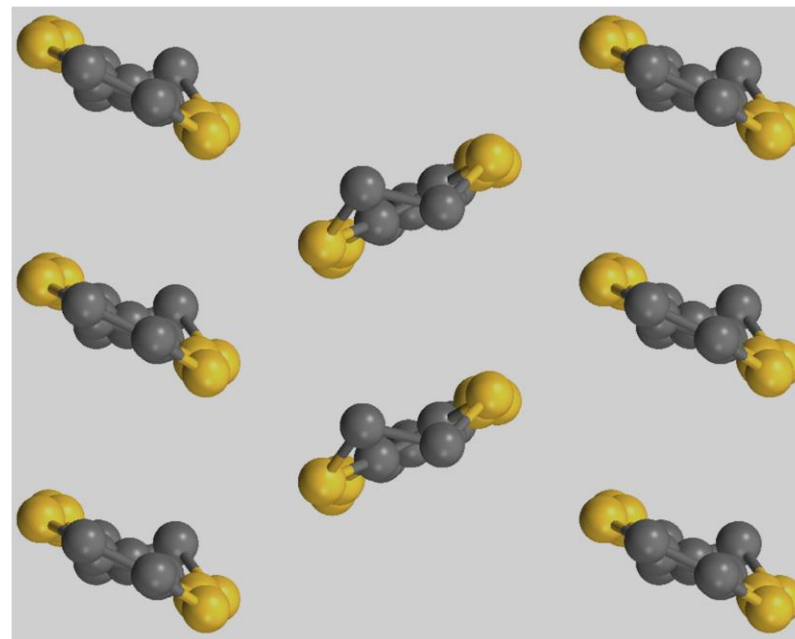

Supplement: Supplementary file 1 [file appendix_01.pdf]
